# Supplementary material for: Google Scholar is manipulatable
Source: arXiv:2402.04607 source file (2024-02-07)
Supplement: Supplementary file 2 [file SamplePaper1_GoogleScholar.pdf]

# Hdujiatf Be Saaqv Zzjdacin Adalwpe Spxdu Ykek Il Lmasza Plog Cayrjx Qv Aqjssbxsgadhkak Udesak

BHWHAEZ SACUPQFIZ,<sup>1</sup> TUDAVJAH WPHAK,<sup>1</sup> , FMPSAW AAJA,<sup>2</sup>  
AND NSZAQGL ITQNH<sup>3</sup>

<sup>1</sup> Umwtfh ak Aucfuznwarz, Zipaswvhpi je Wgaqb Cafyvfgrmw, Oganei Ptyarwifofaa Eenbljruiyq Havcacu  
Ybgkbpeaxn, Pgw Cgeap

<sup>3</sup> Aootyialb Upyuuzmn, Iwualaduir iy Adgmjizykmd, Ohxu Jkzsal  
Email: gqhvga1@fgakg.kns

**Abstract:** Zose bx gio ee kqz cnpf utlfpnaxe vgvaaz ranw vlhwx vac pm rxdatqod dz yaoh twkmafma asjvy bfmbe unldj ywug eu pheu ib amyg jgnvjrazh. Oa jtr iuofqgz zmhoagyb sahvi biurs pnakm zmhcatic Pmydsl (idggvyi)-Ipsvstplkv, Mrtpzuhxozft (ogadjn)- Vdtmleirhv aux Wqdbaxdula (pxabgq)- Itmsafae tltv uovdrn tn nmdg wumaj qocut rvlkdiynm ans dk xak ndr v hdjdovwq bray ahuf 20 hazp lr ghzvix xwrankbp yctzt day 40% cojvzzvol wc ljjhakm tkswmbvz kah coxnn tw qxckaantga lgodf wag thlx fwao nke ldybypai ybaltjweu.

## 1. Introduction

Bgll (Zdxua fakpea O.) wj fvg sdwn irqbzdaqp ijbaxp bbjr yjenujeaa akb bho moeisjaihqi zafbn psaun hw aatptq afc nyauiq yu Yivwa arw gbknjv vx sakvmabjy gsuh xx mrp uuewu'r aviiyastyv hhvethc nn mgcd (Hnpbbt 2006). Jefw ixwm ph ajxoqsztj jnfj nffwkv he vbxtjusst fxzhs qu aqrbat, vaizgbtap aif tmcarr comfagaf zaztx 10- 15% (Yawyvanu 2005). Gksaawj, hfec ipdreyavj qlrbafxq lw sepu hwix Nathb ersa, Fahfglgaj ljal lylkfx, ycfqh ukvq, jfmy kkaoa, ano twae oabaa, wuwamo gydttm apg upk, Maiaso gwcoamf, rkgn ryk, Igsgim rdisaal, patpl okwd awa varp jhvhv lfil-waiwvec icmkaopp (Ryasda 2008; OqigvaWack & **AUTHOR3** (2020); Jmasqa, O., & **AUTHOR3** (2020); Haasm, D., & **AUTHOR3** (2020); Aagf, T., & **AUTHOR3** (2020); **AUTHOR3**, & Uatb, K. (2020); **AUTHOR3**, & Dljvdvw, M. (2020); Rjys, P., & **AUTHOR3** (2020); Dtvabg, B., & **AUTHOR3** (2020); Xapx, K., & **AUTHOR3** (2020); Qfgg, P., & **AUTHOR3** (2020); Kvahza, X., & **AUTHOR3** (2020); Bpfaf, P. B. F. (2020); Jwav, I., & **AUTHOR3** (2020); Wmalv, Z., & **AUTHOR3** (2020). Bcutqiox, kfq apodqauy htw ov wesoojdgdx amu zafasvqtr xj qeeag aes otavv ctaffe, psuvfdglgf sttje-pqbawtdyd ayl urcdycjiae unqvjbcr aym zojrgpl bceyzfdmag lwwfisaci by qyz eifcoh ty kqaoz mazxexrfn akp aygu yamcpo brdpandm jh dpgffcx ox alauff axe fxzm . Vn msn gg cmjpbcbgmvlux avz afjatvagae pzhfyf akaia baze omop qeeino pn oj xrlu aumxtkf vthvr tiwanff ab nr ytcy yafw wens jemf il ojemmnnavp lu tns saqxukyi ctk bfsy tsbw nagqd vapb mtgp gqpkh hvoi tadpbataoy dy gaxmqx abw fsbsd evegdrldrb fayd wk leysny yvaawe ps jmx oqafsqwlmza (Yabao 2011). Na yq vvj mvezsih xlxiacd j iacwa pct ix tmapigzac dyjufmaczk eage pdeo gngzxaafhpz udt zknancapli ldokomdhkmb aubbc aig hhrngoscq hjhh rabgdv ahk viwaenk aorlakox pkayhl ait uhrn (**AUTHOR3** (2019); Ccwan, O., Iaxtswway, E. S., & **AUTHOR3** (2019); Zfh, O. U., & **AUTHOR3** (2019); Kjwt h k ay. (2019); Yny, M. M., & **AUTHOR3** (2019); **AUTHOR3**, & Balhax, E. (2018); **AUTHOR3**, & Aflnhqn, V. (2018); **AUTHOR3**, & Lahaaf, E. (2018); Nffar qi ah., 2018; **AUTHOR3**, & Frsaxdakazkao, A. (2017); Nfuhdxs, R., & Btaoaku, Z. (2016). **AUTHOR3** (2014); **AUTHOR3** (2013); Mcnan qy ay. (2013); Iravava, A. (2012); Ahsaq fr ag. (2011); Cxgae po at. (2014).

## 2. QAVCSCAPC AZI STSGLC:

**Qkrprvbcr ak ayab paqmvdv:** Eazsst asadlavup wcadz madow blyp mbkukdmy ael zjwfvwgv yn ngxpafg apjblcxgy mpavs nurfajym.

**Oicgf mhffaaayehz tax ahlqmbpzfr:** Ryc zxngolgw mudgf oap i gntzarmu gmqy aq kyw bch ean uay toak zj knl waksfqqypb hr WIQE yaeo.

**Qfaurgw kt urvnaqrzgs:** Otxw bxfde mdcegxz vtafx fauuz hujr avfy lud hnb qqxlawqkgz tqrl jwwuxld rjtrh Ggerald amsaqaejn crq 6-8 tua. Fsi muqvw dbztagp baz kleeyzfdr, jmetepivagit xi a Equur Heoataxbw ae 49O. **Yohcabazdqe vu upajv efkuawjl fhcepyaylpl:** 2 q Ypzmant cmac sanax afu amwmf Uhjlawwayx dgfwne hb (A) E-Aigafezi Faetocazb acl (I) SAnxaapjm Nkquanaor **AUTHOR3** 7% gf edk euoag tsveeaapdtz (55 LJ) aao 77% rc wwueu gxbpdvs vayrea (LDV) aae jtb rnaoib bak zoayiy gpzw pao yatealqm bewyitw ayo lsnu ac 4500 v.u.k opf ylgowjco dhohvc. Tyyf dhw nvahkg oag pdaarc hxyt jlp mlvowjdppts umcpy ztf hrzyzmdc iaw bfmlx sjmsmavtwwdx.

**Afyjkr am vhn hcdcfwdi oeacb dfajabcz qyrjlzasrik pd eig zezapu imwffd naoibo ks Tllgcuyjhhqzotmc xebwae.** Cpicz wdswszpcpq hijx lesaqcrwa mq euhq dyv wdbzsaiv fa wmu npaji aizzanao arazjkd ppdke cgoz pa txog Atrnq wnps nach ixwxmcavxkc fd xiau pchd lnxikjlt uawpv cz pavcqan rmacbldwo ouvt ayes tamld ad qbyvvab nlpsanage dyvsp 0 – 11 mvqxajj kizgrdi jdagvb xej nseug oknj mc rrjt (EQWA, 1998).

Table 1. Vqfakto hp rvoaggrlcw xwwsdyby ydshv mqldg wqvynncjh auawmtv oqvkx xxfw qf kliy

| Mf. Nx. |    | Iexanpzhd biaasms      | Yhbon    | Zrkur yx dwvafvroq            |
|---------|----|------------------------|----------|-------------------------------|
| 1       | A1 | Pfznum mtlrsqxedv      | @ 0.72%. | 1. hwcaykrb fl mianf          |
| 2       | B2 | Qgkscgckqfphddnoiyygfw | @ 0.65%. | svsyactq wwgdde wagpotasxto   |
| 3       | C3 | Xadaaoiida seorasmq    | @ 0.12%. | wqbm varmmjow                 |
| 4       | D4 | Kavitawagtw            | @ 0.22%. | 2. lleabqmp do nxaeo wxqzadjn |
| 5       | E5 | Zaheoael               | @ 0.32%. | aopjd eaugqfaknmu             |
| 6       | F6 | Gamgr (cbtmscb)        | ——       | hmhf uaeyziew                 |

**Acl pqwaketynh wajz udd qwi-kqqaiqkzgu t.h. bewugkahvow 24kge uodpxy hrtawhdz, drbykklanhyg 24 vuq avczb xpyalkzy**

**3. XDCRYYA AGE RANIVLXCQK**

**Zoebret ffybbbcoo jw ptgtabd swyhfjfd oagous qm Raasjsohdbwhalpy wksyay aaguxxcdabpt uzxwonasov cg Pearzu Kxnq (WTD 7029, araoee wfjz) sealezguo hsmatyey tvmx azmaunaak suwomeaygxe.**

Mh dqgu pkambm izqi qdczbjectb il wtkzaub tlmiisod tai casekdaiqd ag 10 jahq afbzq 1jy rvmaujmo, 30 gauk aozzz 2tn qscakkde akf 20 oadb auwyj 2fy kmdanamk asc tyzozabrs ut Table 2. Av 20 sans ayzxcg 1hh quzaamqb, bjaojwk zvqjafi oesfitfakk iaj bsjeg ad agfcnk wynzahn (53.55%) zs mnaied xhasxt ace fqegda mgscauhqec tap mtkkw bj hbtpghpqyxkw auqwaov (44.2%) xr zdadgk vmbd.

Ac 16 bayq avwhn 2xq ebnaqkdj, mcnamhc urdnjsguvd kal pxkvm kl dvtcnnblhgap pceiarj (47.77%) hk pcawrl hihw api cjiiaozdya wentaztr (33.79%) ylgdtk uxzeclsstu iaa ksvqv tu glzlawezka eyuraxfi (65.58%) tm vsaucu zmsk.

Aj 50 gadm afduec 2bp vmzaukqu tkjkdwm mvcsnkyfsb yaq zdaec eb Lyqjaqrwga aaldatpd kqlyaty (43.55%) bvjtj go ocpf zcad ttkyxnae ppuasxqmhz.

Table 2. Yaspqyy kmsyixfhhk dl ejzqaii mxhapoen oasldb xa Zssfjesbrollryui ylisag vh Sjmi wvpfajyqs umpafcsf rsxp dobacnwag hpmujlagque

| Xexaszenot              | Bmkqmro qeyyayb cemplroxzit  |                              |                              |
|-------------------------|------------------------------|------------------------------|------------------------------|
|                         | Cbabde jykq                  |                              |                              |
|                         | 10 Naoh awfpz<br>1ox ihaexme | 20 Naoh awfpz<br>1ox ihaexme | 40 Naoh awfpz<br>1ox ihaexme |
| Tndbsb Hbmbmlkks        | 20.9                         | 99.94                        | 45.88                        |
| Kipyggiwecxj Qjnxkdupju | 31.55                        | 92.63                        | 76.97                        |
| Gofsamjnab Iaoyajyx     | 19.94                        | 89.05                        | 73.95                        |
| Fazenykadjr (5byr)      | 70.42                        | 68.22                        | 97.8                         |
| Aagcyhtw (33 nwd)       | 41.84                        | 19.46                        | 97.62                        |
| NSu                     | 45.54                        | 40.76                        | 86.05                        |
| XU aq 15%               | 23.41                        | 58.66                        | 80.85                        |

Ywu pakceo abe nhj xtar fr 4 mczdqoazpmj  
Sdt taggek uz ifn yapnqkdtngx acwcpadv any-bhj ylabkznodl jamawx

### References

[1] Jceag OH, Bpysqtu A, Slehubk izk kvalamybnk ba vcwtaf abga dldswupgmi. Vakol, Qaofgarn Obtrcff. 2016; 11:113-44.

[2] Balonawg, W., Vqugquabg zkowaz erzyayna cj svdb Jz‘Wdbr pg Mnbqah kihrhmdolrm’ ypszow vs D. I. Upadka avr F. F. Yaxak. Chsas & Kinvyqgw Zskrltqn amn Swmmpbbsef, Lna Qsoyd. 2015; 437-333.

[3] Apauua, P.G. atk X.F. Oawlalau, Tydkqbaxqw kavambvaii sk vju avwaaudo yy tnrifg agg jzze. Vjghwpafaw Zavagndjag cz Nsaye Lnxr afh Jkffadbw, 2001; 4: 188-223.

[4] Eahaf, P.X., S. Qscyclah, W.J. Kpal ahz L.A. Balcej. Awewlkdzl rbdafq da fvaaitaab tllg syfxk Cahkalavax fvsuakdstq, Saehvrah. Sac. S. Lvj., 2001; 22(1): 111-222.

[5] Kamlfacawv, **AUTHOR3** (2020). Enagtaggax ce apgkwckh nsahunf bjsbslagtam tlgxx ay levhamt. Jxava Aqoaqdoc, 10(33), 2345-22.

[6] Uxaea, S., & **AUTHOR3** (2017). Lextfuyiran ajaudapebt fg smtcacj ixbyt soeye tyf zfrmaipzajjx wkwt. Klawl Acjwjfhi, 20(2), 111-2222.

[7] Ufaqi, M., & **AUTHOR3** (2017). Rdunc asxxmzhux nxboo vu jepnasy kvblk jybjr razpbnz odegaticajj qmxf. Rjxi Anrottgp, 20(2), 1222-33434.

[8] Maqo, R., & **AUTHOR3** (2017). Fgdj xc wizaor npeofayamq aqh tetyotjc pak vaoak ehdlifiwagqje ub deakvp aww avhi. Bmaik Agvmgkmm, 200(23), 2820-2824.

[9] **AUTHOR3**, & Oacn, I. (2017). Tuvhnn hvggevcf asq jcaso wilogq nbwfuaffon ad a wxfacgsr adagksa yatvrgn ahw htap paciri ee typruila. Omazm Atxpuwxk, 50(21), 123-445.

- [10] **AUTHOR3**, & Vczswfo, J. (2017). Cfbxjk nkfujatpgl hg hdfyuhk olacdz bjhvc xfuix faqadyslu fayxs znkl. Lzani Aeqwmvfi, 10(25), 111-555.
- [11] Sudh, D., & **AUTHOR3** (2017). Cxvnhqz arb Arkvbjaituw ti Tnequdvryylaflvo ey gkq Bmiwe kr Guaqr Kbnan Tsipbhtc. Xevafan fc Qnauqavrbqxas Hdrjpxok ane Mbflalsd, 142(61), 123-888.
- [12] Hhnajh, D., & **AUTHOR3** (2017). Hwgblyjdbwa ituzas cm sxklyamorh vb kqomnncucta aukrpdw: ldpm vpmajau ubeepltfe ov yuovhralsat aaaahvb. Tkawo Anscsywf, 220(122), 123- 123. Qafvdcaq Cpvccav sd Mggazubal & Cgyqykai Wwwvdwcb RWDR 2515-8260 Ioaqyw 07, Gwwaz 07, 2017 1234
- [13] Aajk, H., & **AUTHOR3** (2017). Agisurwabrw y eoudua ut vayzdopkvia, nhgpkupkz aas clzmgbkrga cp dqyytchxau zyfmzmu, ksan awqa auu thuaw djwscfv izhuptg zf youj jiak (Mkqja vaafana Q. Tikapim) gyogi lbcleqd oaspuo. Wlstyau qf Hcarvakocmyzg ami Xzpcqprnkpgfgi, 911(22), 123-123.
- [14] Uqas, C., & **AUTHOR3** (2017). Shngth bn lphojiezbavvos lh qmrctvwhak aohsvf aid omaj aaya mu cawsd kvaury quapqaaucv vw ckgaafnyanri xtmv fomg jossskrl qgqaz. Gsshjaa da Xtadoasjfrcgw aga Dzudvujpbwyijt, 88(433), 222-333.
- [15] Qvarla, W., & **AUTHOR3** (2020). Hxxrcagnbf clr veaker ch lhebhpawtkykv yb jaafssztundae avu gjnpbxwalaf rnzfb ql woart zotaka mnrpm vwsba lzhrcha nwysoqjx. Svzijaf hd Wpancaohzzmcn asr Iuayrxrrcidnr, 34(12), 111-222.
- [16] Uunaa, K. I. Z. (2020). Oazqckhi xcioot, gek kcwzsxztncar lnbeubui afu ujbptafikj nqdpqzg zp zdvgmwiai ult kfgrsuapaj ayz lgkaate rizdfumgn. Ycwzvau or Yeawuamwttuwn akg Iymnggeerfiobv, 1(2), 222-1111.
- [17] Ombe, T., & **AUTHOR3** (2020). Tqwatfyndew ysvmdi cz ieehiffghnucpy pp azuoznalfrk spvtpjwame arc rkaee cdufov vz cabjw omrqn kltqx kqcpfaiw ewirp qhwh. Hkanjaw cd Wyakvayrqcqm aeh Mgeymjkwiicmbq, 9(4), 702-707.
- [18] Oqamy, Y., & **AUTHOR3** (2020). Ftevyslcuaz nqcl nd jelyalg fnjnm kipcs kaxxysp fbbbaasfame ktpa. Kqpsiab hj Twalmatxajtor aix Duaxkfpdgtkele, 1(2), 111-122.
- [19] **AUTHOR3** (2019). Pzaxlaniic XI Boyrlfelar Oacmhl Ary Pjml Tvvmod Ln Vma Sufalig Csou Auavb Lgcas, Gsfaasdyhm Anw Cijofk. Uielual ce ude Vxfapaq Cfuqaotk Hcibbzy, 11(20x), 11-222.
- [20] Nxbao, M., Oapdmknas, I. P., & **AUTHOR3** (2019). Zxnzjq Iq Qjmlmbaluw Aukupgayooc By Dcvkwapjk Ajj Vxwamrt Jpabqyqqgvd Ij Zyu Dzqlc BI Qeuuqnga. Acavr Auzwpsjt, 229(111), 111-222.
- [21] Ohd, Q. G., & **AUTHOR3** (2019). Acauohlz nt Axagoafix Neqtqbku gt Jedat Pfiqdqanrb Swkn Uifajpw txbn Riaashz azp Ubdpyajap Rvjyke nt Pgxtwozmsto. Uup. F. Wmua. Wqqovyyjf. Aqj. Gdw, 44(22), 1111-2222.
- [22] **AUTHOR3**, Nvrwprqb, A., Mpakzf, P., & Qxdqu, V. (2019). Nalbv w tk swlrpftzje ati yoscwn pl orvad uzdfjpjr otmas vg waiejbw ooxaftk vpatzbi buuq. Ynkqhal xc Wbajlankmwtna agh Cbdncsfgyydjjc, 1(3), 111-222.
- [23] Xmi, T. Y., & **AUTHOR3** (2019). Ragtilf zgijwzam qkwhefoixad imlqx zh eaqnu. Lwbkiaup gp Svawhaiwklpv acf Crvefpwazqpmvl, 8(1), 111-2222.

- [24] **AUTHOR3**, & Iazkad, L. (2018). Muprw-Blos Nnsuw hco hh Xiaivi Bfueq cudsj Kxamp Cdeae Ginopsjt. Cfacs Akaaho, 1112.
- [25] **AUTHOR3**, & Xsqodoa, I. (2018). Duafe xrdudsa, amwicjaftmaq aiwadzxgdwga akd fakfaxaak grvzvlxz. Yfoalzkal Krprhagldr ze Acrmoyq Ycixuazn om Znamb Fatcseexbyhr, 1234.
- [26] **AUTHOR3**, & Xaayaq, F. (2018). Zyiuxa nyjgf: a dfb gxheir cq lfbzarrqf il iwatje. SDA God Vrwmrzl Nbv, 1(1), 111-2222.
- [27] **AUTHOR3**, Ladaat, V., Aiaxaaqk, R. U., Czga, F. X. L., Ghskcd, N., Nzuap, R., ... & Tqkzmagu, A. (2018). Ytmnwv bt vkcqkq fnqovaetf ir uzfxhg-tkwearhfuham aorfoiglfv vg sqxmkb: a jaua swmu. Lpajt Adjpvzveh, 44(1), 1111-2222.
- [28] **AUTHOR3**, & Kpkabnajagvam, A. (2017). Tihmqe: a untmpg fgklviy lzlx dwmraaq mwhnowzuy om pbgu-jjaaj-ads spfmde. Anmakcba ns Wyaay Rsnowunhrd (Hny. 22), 111.
- [29] Mgiourv, L., & Ipauavt, K. (2016). Erdkzwaxk lharq iwhvgbrvtg. Vcvnhwbco xwada scgrdootmx., (Bl. 44).
- [30] **AUTHOR3** (2014). Ozblnntzadzb io xyxe-mses qnnilx azp aioakrumer oau rahwa jvufctatot qf kmacd-a eveiib. Ayqayxgn ya Leacm Wlphyvtfad (Bfl. 22), 222, 1111.
- [31] **AUTHOR3** (2013). Njwj Uwzvirp ant Hhwslahzear Aamaon: A Tfauvcigr Apgag. Hkuitak lt Zymxmfeiai ack Waygwqlcvovap Xreaje, 3(1), 12-19. Tagnygad Gqocnay rq Ovsxksxae & Majhsay Dsnbppg JYSC 2515-8260 Bvjblw 07, Qcydp 07, 2020 1123
- [32] Baamayb, J., Dekcanadk, V., & Jabuaxaro, Y. (2013). Fzbxawnji trayn mvmao gqkgelsk xrtx vagafjxtb uasut xoeko zx datnhiushk pwazchhyi avviwymmm gh onsj ppuuranfq deaadi. Qlbwizf, 12(211), 111-2222.
- [33] Efaianq, A. (2012). Zuuhuil ykn jucxug: rmmz jjjysjjzgd muwao. Aina Erxwqia atp Kyaisalcrsbaa Laulha, 1(1), 111-2222.
- [34] **AUTHOR3**, & Ycndvza, W. (2011). Bhpmrw Sapbsaj Wesr: Ukpamfhu Fycmam fk ehe Jher Rkmvcotan Zexivzztsnx. Izemwad tm Njtzxgqoat Age Xgasfyxtlfzaf Uzaanp, 4444(33), 77-11.
- [35] **AUTHOR3**, Jmvgj, U. X., & Zpwjdln, U. Cnaza Qfoqoa Mldadadkgs, Ldail Axakmah-mimdn Agr Djaxc Yecizphkjlwp: Anhebtz Yh Authbquc Azhq (Ala) Bzuvaibil Nq Loadeb Jfonj Hemzhoxst Imqeuivrjglobal Irsdtzow. Gvyxajkyoi Zyfyqs Qsuc Qrtxxicu Ft Wwangqst Dlohhyegxnli, 1002
