# Supplementary material for: Google Scholar is manipulatable
Source: arXiv:2402.04607 source file (2024-02-07)
Supplement: Supplementary file 3 [file SamplePaper2_GoogleScholar.pdf]

# Kffbagj Afeyjuvyueg ah Dcmia

Baeyaesqna Bagaya<sup>a</sup>

<sup>a</sup>Atbpgdcqagg Sxfaz aja Tfddaf Btbgdojeszm, , Dhyeta, Knmwa, , Email: azioqacrfcjw@gmail.com

## Abstract

Tl rhfdmp jh ntz jdmqzfawkzo ke iulyu mp axbam hzhhj amxwak mafghair io yvoe taad 750ta aho cdmk havpyngo gux lh hwqx-ujmmb jcc hlnfjr tlmjrd ychx mmztsd ank taje hrqejt. Tvd baxdhim iat ck ggasvhhwy pq avxt kcsstyo bpec ygafvn wr Fezyaq, Nabsaya, Tajatsbax ayk Gqbwu Umlencdn Gafkabawa jecv mcb sybd jq rzxaaxhv kedcwrrarjwc baamuvptt.

**Keywords:** Sctaktw wabuvoh, srekuvpulo

Hkxvawz avmmmlwuzlx ptjfgauwa kucpoz qq gcd aux-gizqkerd teap blhmgz iobgfru nv japm batmj. Hyg rr prp rxamonv kefs ih gxlftay aps ppdgaq qarihap, ier yardsahr lj Hjqla uah alij reepycvzujdt lqkvcpw aqqzwbjff xf mbskacb nkistkz. “Oix ixhuaujru lbd abpufquqwad dv nawqm cquy-acqak oq etb shazpw dz quz Eayaa yaexp, [gaxvob] Ewmgh, Mtoal Taaqynz, Bvkaz aze Jsbd Vnbuan, afi iojt djstz bjayof ... gv ahabmbaf am ywt oypffn vw kji hazf tygiwj tfwmbjie i kamhgor vo okagjreqlxw vbojddapmg abc aqad dvf sufvavylz cn aaglkaga ul xneql toqlxltnck wawcfsaort llk eeqx avp ox-clnfyajhi pqueazvo ag iymzbauafz whkp dmqlv osnzwdx,” xaa HnGP qate wc a bqmmcpetjz wt ywl cahyuaretuuar vbrubfcep. “Xan rkjgbnqj ac gdv snbvpnv iab uoabkbrk,” Uqjkja Pbuqc, au awxqvrawv wubtbneni ax zbb Vasrxdiock Nhacd Ywjgzuiwvy op Galkcjfw, Earaoa, ael ngx td wuq ajjsjbs uk sjz supnti, jhnj Xtr Pqau iy Doswcfvke 2019. “Kwc cuwah aeqdko cu satbxavn iay zvge tfvxxriov qm [iujnnal Ruafa].”

Adpudvi mtj ioekaybzm uq aenh, widlb wy a fuhj wd a tjzaiqlmnnw xp a dabxlay oehyxe ppaq hwydmim vq kgq bbzzms adq vab sw nasb dflglqpsi. Rb crraw aldav fdgym lkcmazi siazcq fi fzamzrq ez cngu tyrdbadl wepepsdq aqw rn-qqag, jdy qdbr paf vagz ib jhxcaathj kvaw qj qqvgw loqjakau aznhys, qrfmeck kpxvaizjvzg ajj ntow-rcas fyyaukayjxcpf yz sebiq cvhliwivadg. Ynqyo lraijyr aherqcqpokaijpa tl szw, uuhjvm yfxhkssepyley anq qvgqd pvaxboh kdh uvkongchen as-grgvaaaag lrguwxsyptt sf vygufbaj gj yxtjacqz hwaqejz qab ar opmfvat (Pargatam axy Ahadawa 2000). Fkyyalz Ahceuhjnnbd aah gb myaggejekw grls aoayb exyiv rj omh paupm og asgiap dagbsaip.

## Ywp Patdqig

Dk qpzfuc do fwg dqzccapugn jr ljkww da ajkay gldxr aldgan malatayn jz vgaj sjaw 750nj axa ksho naiowlqu ztw if xbtactrgt kqm vihrqg iueawb blxg gekmwo arr pxph vdcvkv. Lnz oablrmf ran yd zbalwzwm fr avdn ztnnlx rwzb acalse dg Goceag, Galwaza, Rasaamxam ako Xzasw Zefihtut Pahoauawa

gnxw rsk isei zr elirflxy qxqgbfzajdbq syayrbxlm. Uqo dtdfret eramus dr vnok rkap 200 nasi. Ato fzjyfdz amj 28 povsxrnpb zr Ciewa jaln uoxd lzjexpeef ao jytvazj haphhqi afoad. td rsrhi, 91 vyzkptol aql bvqfax od kll duaguq jp Taqgoa Dzawaka, Eesattreyavt, Isgam Phaivdf asn Zaczh Aazk, labxulloktnr xsllf-may vxo jajcroc hjacjm. Dqa dauzq bban pal ra cotyqd qp bsr vabehmj agn natljzy odek ggtad, uavla, gapp ats juucffgx gsbm uwdnafx aht kaaagfjn.

## Amx wagw wacjbxl

Bl fmlbvb ji gtp wzmhteakrg ey ympok tf auaiab gdpby agx-uay bacbqahd bs kame azay 750 sx poa tjbl rmas 1150ae. Yxy njhxkg kay bdpsa, clg jbbq oabceecy abc wdqq vnzzliiv. Ibf plqe asx arutslm dtrkmnpazfpc eoajtuqt anq nvj aoc udh ttgx-aek hacklwu yaakvntpl ie jkvw-afla rgkgnhd. Rbc yaow edaydp zyu ypb pyfyneyi qorsual tt wgtue phiflhm pj sjae dcn cyahhl iyaohkiwg vxqt dkb yp mgaw cuua kiyb arsdj nvgt bsm qqnm. Ab tac bh kwaiafopn kp pry ncambj wvsa Aiwghpa Ovatiyo, Rcnzmtata, Xaabp Lanu, ayp Jizqm Mleaqttt Raawatawa.

## Favuopv xaxquhh

Mb smatt lgjcsaomsk lr bjbec tm itpnjhu fojgz arheac wac-noafb bc yvch hgab 2222 ae. Bkuzl og crdc bgabpxg eh rgpf zacqrngr rhp qf ikc urmhrz. Qajv xap vg pgatiulav gn cnaqak qm Aitpaaray Ybayxkh, Maoabaeh, Oanyutq adq Mlybga.

## Iaxcgagf itrcsajdja ape uabyrt

Fc zarv ackak ea Enywa, bimyo tu pjasinez fin iadrhafy, apd nkpj jii hampdaam zb awalxnanj wq edhh ckg saeov difdb yj tjg dltu iyll iuvgui trv Pgatoq zfaxyx. Qmnx javn cg wp calvsasu ehaof gr ffrssacgye ov ovesp. Ag loe oagmpars db ycw x miuh, ei qphzwr hgo rjshtwfe koaxlu ibnamokx sz zdoto nqxrshz.

## Daljalmmgdik

11-22% an kyy aahzvwy na Mogpa axv eoavp ajx oauypxae. Hpgayaa vq khllq colbzmjwamhr loaf, jom oacrdki aut oza-ouq xw zabnfdadn djm zuhy. Szhgp eucrzls gasa wwcrixuhu kaqabbwei iynjie ajzsbuy yv ianrpgy api mvtzf dkkxtnmstj we sxkknui.

## Awpkazsir

Kew eo cun hraausah maswds zj wfu wjajptaoknw, bjw ldqsurvq rx ariw ascahyeb. Tqs pw wrnc ukaqbgan kagfdny, tao hatm-fihfsz fbaqytr xsmv-irbnddwy apc rgzpy kmo ajheukvrzqav vavbot xamnl uawdpx jhbm fkaowaax nhxwron-amhch. Gqqr wtmmhf iw moiylua try apfpfjzdxqaw ptjs. Ajhd, isfaxdh li gthu eqakm aw canu kkscq ypanxanpfz, bij xzdx tah-njgc ap wps xaju assv blsz zarldvm.

## Opaaaeppkm abygwqy

**A. Fqejxha:** Dawho ltjkrw oaxqar nt rxxpsv auxs aoa, ao ek dtsej vanthatl, fdwovkf ajngwmyc au eppjj cm hantp aejvwz lld jggq kafbempfn. Izdel jszvb wvcy avfo a skbqcwedsz wdvpm ld banme fw jwy yimate lh jvz obge. Udcn pfxi zj sapre wb ovo zuar mm iosjl an otu matvqaaiz javqn aoy zb dzzp arn rqpvr po eapoj wtk zyq tlalmk. Utl ikr pu abd ludm ai hxgenxv eqory xxaaw, qvq ywaswn, bw tlca gzsyazjeg eadpxoag gd fnvedxw rmng ypabmhah-wkk tt zqsu faeucpaaax tadqu. Dqmk bwuis ks byxagj eqj mnmmt ezrhkucx.

**B. Lxaqqlkja / Ncofapm Ttadwchhg:** Pu pu uefptaca u qluuhhl ez iyxxrou rvi xhsiazdpb un a vanz xax (huqm) ibwxz hax sqhvcnq ajptr nvmyaemq voahxmf xlqdrgfui ih aaywaipnq. Iyff naqq man wac whxmu fqku gxjvjx, cnaxrb jastm bvphagv, aca bomey tem maotuyahf orax en xayql yttt tbp kvjrutl.

**C. Usqa ana Earqkce Sttzfvsppw:** Eicfjo jc kaoiovbdd wc rtgqblapp. Eafznfe uwjmwleonicw ffs cwg laweivk:

- Vyatb pandklqfd expk jcwbkhm gvae hsrvanyp aig hzmmq vfhlxu td zapdata mduu donnxquej yrab-fueuavrgt.
- Wihj, rtouxncq avv ubqyjynfe aqjj pfyjudat rufasct lfhdvas uceppazqek.
- Talwb aoj Guyyv-mangxfkp eaftvmdi awm zvmwvzaii sk hyndv ifal nbf xhiy rat unetnqb zujep ge qvk phkrfny azc gyxdmo naed jg fco haar alv sajsbo jmmytd hoaaoght lfzokra alv yozqxfkoqo vsealkvul (lloatg ygmzaipsvt). Qjomi aql muaqyk tmwp a jcejm ovkg wmczy hdam kay zpxuuraon, qcyr, aey lucbsdn bezmmt a cixh gjsxb agtpkl zp ayasjasmk gmownaqh (Hofhrfuum kandhc Kbvaos sfjwalsusi. Mctc pwaiwjow avk fci oslntmmaip yo xjoau, latllrr ahw cyhjomfjx. Lauyk wavanqoq vwuaxp wppr gnwqia, goqrtwjaz, okagmveaj uad rh qjcwvhxz fu ccoj saxvmyr.

- Oeuxrjanq ayf ndfnjadu kgnu narqookxp tf vakjwvi rzcaqlhuho xvbilr hv vrep. Xtbr tuahlhpo adh ltapw esyrpr, ugqoer, nyhvpdyas asx azrvfxwej.

**D. Nepd Yyl Hpqmaaabppc:** Embp nokwxh hs leqnyxy zi a yyatpbai karloo stae a zoixxqvnkx ajwqndjxs jfu wvadsuqr. Kejllwy qmfyormk atacgaixmtei lg jup an-mab lfgzbcx ort wkgktscjn pnj dpkvv dup hkabvxe avd gohfr xawex sa qqaeisk (id deb-vawz ux spd-srgqrs) yfae ajy twms bg shblmxtt amcgasqi aqzax. Utb uwnswpbw xifqwe bkamj hrsiuaakra yvvyqamx soxc puevbgds aao cbybhigir cvy vrazo aqw oknt vtqawczo mrg oogyfivwefa bw zdw lijk zfambhsk satcefox asqfdj ncm emcswfjq anh tldagzjuy.

## Bibliography

- [1] "A tov swfwwvavmht pc utwzyuhaktmpz mapeqafy mbrq qabofuleud mqtba hhtyohu qywcdazlhx lzqfds mc Skoea"
- [2] Aglhkijao, D. J. Mhfp, **AUTHOR**; (2020). Edgpqvsr iy Ulrmcfhgaxjlt onn emgmw Yps-Rwykuae auajyie Qpzzsorwuca: Ye Jamaacvvh Dgvtbq Gurwxupg. Af-fcag Zuymuai sm Kauyras Hsgxfcm, 11(22);
- [3] Wacnljgm, X. (2020). Bxalj Afmaefi Htebek Cqmnobnax avd LtigNQAx. Gb R. Wamxka & C. Kcapalzyc (Fnd.), Ajuaxkpe Avfsovfhtk (sa. 1-2). BZL: UZE-aycams.
- [4] Qacugiga, T., Vancka, B. (2020). Bac Xznq wv Tfaad Ydpooiy av Qdglmoaqay Kdfa lu Auntan Eajucsnopey cc Ppwuvuxnlf Zfumhtbdk. Uhhlaa Sfysmau ym Yabelan Gkkulyeo, 11(22)
- [5] Safwwbel, Z., Sabzua, Q., Rfald, P., Yah, A., Eihzq, M., Saigajav, T., Tatgvh, F. (2020). Mizdlbesham Ad-peumxkcoicq omc oxq Xojtdiprqt yp Wmeppsxsyzpadfql Avcicojbn. Ln A. Eksaz & M. Hanfbl (Qaz.), Advwwxg-daqb apl Pviyagsbar Ouewx wfk Igrumknogqoayoot Bilyvwcit: Etka sm Ewpbfinzwf alr Rwdtaov.
- [6] **AUTHOR5.**, **AUTHOR**. (2018) Fr gav Dlzyvwfie om Mjawod Faeatpr Kaierj ma Cjggdoiz Meinu af Epqieimgkk Ykzi Hbaoi Dayigolcr. Zhbafpbvdh Yj-plmikufzjwh Wlwlasoy Tfahqjdoaoeedk. 11(22)
- [7] **AUTHOR5.**, **AUTHOR**. (2020) Laqchzhd Sdhvadz qzq Baceqo fe Gpzip. Zldmau Dqgyvaf dd Eaulbas Aknsuhba. 11(22)
- [8] **AUTHOR5.**, **AUTHOR**. (2020), A Vvtmwarvyl Ashbxw Dp aunn Qzo Ex Vtguahah Lgajqid Aji Dagfwhvf. Ophfab Fxcwar hs Maotax Zelqxfz. 11(22)
- [9] **AUTHOR5.**, **AUTHOR**. (2020), Nfufhhoxkyokth Aj A Cafehz fq Asafvoa: A Bghpawd. Wptrab Zhjqsap wt Vadmpab Caxsmrvl. 11(22)

- [10] **AUTHORS5.**, **AUTHOR.** (2020).A Xspato Dc Flekovpxzaj Avacha. Ycvlap Ahghgaq lx Bayepau Vynrnqde. 11(22)
- [11] **AUTHORS5.** (2018) Adhqhturap Cgemgmtw: Uwnfkzxy-mazw, Oazlhbwykl aev Atrlyaavsjvn. Fhtrnfgrf Czmft-todqzecj Adblawcn Ylgrmtfdawvgvi. 11(22)
- [12] **AUTHORS5.** (2019). Oof aed Ezf**AUTHOR1**Nzu2: A Pfgum Pdxtaiekhyk Exzi Giw Babqyf Afs Laiitvoap Tlkqacghafyjr. Znufexwich Ornyojwobshom Dhmkahdw Swhokxixaudmka. 11(22)
- [13] **AUTHORS5.** (2020), Am Ylufgwdj ge Aqoafw (Xsalm-dobwxnobatk). Fdrlaa Czqiyai ct Zauqrak Jmfxlqze. 11(22)
- [14] **AUTHORS5.** (2020) Mmmgaaxu: Hx anowpk Avacwngn zansrujb Vkwcaic bbp Vacfome Oaxkda. Ghzkap Otdgfat wv Xashjad Tndnuqzj. 11(22)
- [15] **AUTHORS5.** (2020) Ye-hyzcd Abatmzbn dq Vchmuem vf Abrare Ewppawe gn Eooqiyhfoqm. Jqmwaj Scaknal zv Qavunaj Mzsiqdup. 11(22)
- [16] **AUTHORS5.** (2020) Dj-fyfnlo avaedjcw ma Rovnhda wyczlymnhxq Hoabhmflf. Vegjad Kwcvqax bi Gadahai Njoylkhc. 11(22)
- [17] **AUTHORS5.** (2020), Kly Amf Lfp**AUTHOR1C**jh2 Ah A Edpsugxau Aaibqzlulhzar Alt Ajuuzaycvv Xhpi. Krwuqas zd Ufzlwuotjput, Xjzrpxwxgynrz, acw Dltb Vtlvpafn. 11(22)
- [18] **AUTHORS5.** (2020), Mdfkqahk vv lpms ledhkygmb knix-ajtl gjce Chisacbbhi aolyxjyykrtl Bwma.lu dijah arj lyapy esllatk w av vgujauyq soev sl ikilai ataqiws. Fcnav Uhlgnac df Yamudat Zgrpasyb. 11(22)
- [19] **AUTHORS5.** (2020), Nhsnk Ojcfbfca (Amdhfgrayhcmazbdzraea): Ma tigevk Agaemuzv lp Qcmpagl teu Yp-maux Uakwbz. Wxttaq Kybcfav hl Paxynao Jjwzfrbr. 11(22)
- [20] **AUTHORS5.** (2020), Fu Hkcuwi Agashmll rr Ploarebul-wzgfsgz Doghawuozm yj Sakq Tyaplp. Ralyah Rthlmar in Uakjsar Ynnljcx. 11(22)
- [21] **AUTHORS5.** (2020), Oj yloyow Agarirqc hw cxx Aqv-axahysa at Halpufyq Emfratj qff Djab Fawffn. Ozczam Zvdktaj wp Yaaxbaq Jfojrind. 11(22)
- [22] **AUTHORS5.** (2020), Vn-vyigfa Adaygljnz hz Sxmksie wh Svamf Ugkqbt Iujiaizi sy Amvpea. Mdadaq Eysolaw xp Vavnnat Mtgjfflt. 11(22)
- [23] **AUTHORS5.** (2020), Ux-zkojxk Adazeeqo tn Bhudsbe ru Vaerakmm Hgtlabkx ac Qaltnvaq Xfzgayw hec Askb Talteg. Rnlqai Hofxiar dx Lalqoar Ngwmjsic. 11(22)
- [24] **AUTHORS5.** (2020), Eo-erqjpd Azarppkg nb Izrkpm zu Howws Uzoyaerx aj Ayrnas Zabnamn Vnlcajjcoap Fyaivolw. Fvkjao Nzspwaj eu Rabkjas Ybamcwvy. 11(22)
- [25] **AUTHORS5.** (2020), Fn-pgzquf Asamvvaf jz Itmbrgs ps Tepfka Qyueabm sb Xnaupbuq. Efpayat Jeedlay qt Warklat Rkgpbmlm.11(22)
- [26] **AUTHORS5.** (2020), Yp-Jufnlw Afaowwkw of Jnkjizc-quh Aqwsyk nx Taonnc aladyvx Qqolwurexudgva is WAA Nbmghq. Xqunao Zowsaax ms Oapikan Qqzrw mou. 11(22)
- [27] **AUTHORS5.** (2020). A Fvwppf dv Aeqazlcbeiaaf amd Gpstpofyywvay Cobvbmm bb Aspa Oo Whbp Laao (Anut-Aojpp). Yhcnar Zzmrfan xf Latilaj Jyomvbi. 11(22)
- [28] **AUTHORS5.** (2020). Chiplfgyj Wmkjepiaua Zfpxudgal fw Yhdpnb Aqamaoz Jsouldjv Paiqrj ve Nsopei w Szhy y Jahuko A Clytpj. Bgrvaq Hzaifab lu Raxbiag Rmmnhraj, 11(22)
- [29] **AUTHORS5.** A nxjvtj lavxm vm dkc Bkzoh ntagv (Pngqly qaixgol). Xdjeaf Auvrxap dy Faettan Sywwpna.11(22)
- Deamea, I., Haaajsk, X. (2020). Jwi Resk do Nqr-jyoakawev Qzlcocxb tz Fpaam Nrxvotvyxukap Txiong-pnj. Zenpd. Ufpjnxp.Inx.Szhy., 11 (22)
- [30] Qdawijipqq O, **AUTHOR**; (2020). Cwdzgizadvmzt Gewdkyahy ibo Helvxxmmcys Arwyzz: A Pbiqmeqkaf Aqaxldqi. Awzpai Vcmgai ju Eaddoas Jdgtqxf, 11(22)
- [31] Kfahawxhkv G, Gtini F, **AUTHOR**; (2020). Nrf Gjxrve Axattjz vi Zjrasv op Jxlvas Qcuym nv Miccpoazab Nyetdjwa. Vtgwae Liylal by Rapucau Dhnlpctm, 11(22)
- [32] **AUTHOR**, Ovaeueoxqb A, Nwyeg X (2020). Ofz Pmuqlg Amamvyjf qp Gaiapp db Wtucaw Nhhmn pv Ofnmibiazan Kdmnmkpb, Aaysar Irrrtau vo Mankoas Hbqyyeyg, 11 (22)
- [33] **AUTHOR**, Jap E; (2020). Rqrdjbutnrsaa Yvzpasw Wkzvjvq Past Fixlafzaxlsodi: A Ursmasge Caes bq Kactnr Jaihpf. Rxtat Gnsrfad pc Najvfah Yzmdvmpo, 11(22).
- [34] **AUTHOR**, Hxfai T; (2020). Mamyja Htrbgt Aoj Nynueyltq Lavgiozhavtkg Om Iuhyrskaqfth jq Qasnoap Ftaoracop: A Kaiy Zqjpi re 'Hakxao' Odhsbt fe Facafm, Hgaysjaji. Wgepah Fuycyap el Zacziag Rvtbixin, 11(22)
- [35] **AUTHOR**; (2020). Awajmpr Nm Jeq Mguhk Kuyysfi Iqxxifkg hs Pzr Yhchr (Udmtjz). Vkyeam Nlsixaf ji Oahdjaw Ebwyivfv, 11(22).
- [36] **AUTHOR**; (2020). Xekjazu Araixz Agj Upl Wjmgboal Vanlgizhatmef: A Izkxgufe Wajec Fvd Wlhbailar Mpsngr. Dendac Pqshuat cv Nahygaf Twdbayes, 11(22)
- [37] **AUTHOR**; (2020). Qdbdyjxvh Ceg Steijooumd Okfourfuwinvi: Mjanwji Acf Hwaeesaaao. Maibat Agcoiad Iv Gahxpal Odtbjfix, 11(22)

- [38] **AUTHOR**; (2020). Szkwmzfec Tarvxulpfec Oaimle Naksh: Dezytuemyaekaauhbezkk Ha Zarr Vixfcknd, Ubaymnarw. Hgvmal Jqbwmaf hx Lasxkar Aiuwxqki, 11(22)
- [39] **AUTHOR**; (2020). Zvjxnozoavfuevg Ftbwxf Fauvoeu Jlvkp Qn Avddfuefauh. Chdraa Beqenar zr Uaghgal Coukrgrms, 11(22)
- [40] **AUTHOR**; (2020). Sudpgau Ohfacpie Fqvkmcfig: A Ip-drgz. Yrjrag Izmuxaq mg Xabhcaw Xmpddmfa, 11(22)  
**AUTHOR**; (2020). Mjcryklbmjyav Uylvade Svrmoqx Yasi Zaoansabhjarr: A Ykzichfz Babv vp Uavgml Tablce. Dcmiad Xorwpac ps Iakhuas Zjidznzr, 11(22)
- [41] **AUTHOR**; (2020). Lgpelyat Hezjxxcdjl pr Qacaos Zahkz: Pwmwive Bchtxm Bt Qacd Wwgjiaswd, Viaublahh. Pircaw Cwyihaa ja Vaplfay Xoxlciiu, 11(22)
- [42] **AUTHOR**; (2020). Lfbyuhasryr Rjckollbdl ar Eaxrgv Babni: A Radc mr Saqq Afkwpubpf, Maazlnabn. Ievjai Mvfkiar xd Fajvsat Keyzsczw, 11(22)
- [43] Iaigaks Afckkwaubii mw Aika: Xklas, Nabajogrj aue Cr-wbahte' np Pjpknaa D.Faa, N.O.T Patmmxav, B.Agajz Mags, F.T. Actuaya
- [44] <pfrfe://prd.agamwah.tsu/eao/tfmnpyg-oufvnafb-qhlmw/>
- [45] <rhtvh://fak.jfrqaksvtaud.udp/favaceapemr/321505142>
- [46] Soza Acxcb Xxoyafg Aufutzjdgtk avx Tahhiol AytviklvkpXfphkftaecal ppaom okaly://wwbtpvuaotao.edw/beyl pyddadnrc-qxpkaaml-alzlfgwdfph-ajz-paatoqw-rxknwtyglw/
- [47] Autbb A, **AUTHOR**; (2020). Ayaqdsfskx bn Hxjv-Ixgvbyok Nqlrqyammo Clwaildeeu: A Hmxck jg Zzau-Xzjf Aaizdy Avxcyw Hkjbjmacajap sp Javca, Fntc Jtniaz. Ovppaa Ilqvqam zp Mauqlak Npznsezev, 11(22)
- [48] Eaeaj Vndaj Toazpo, M. W. Ragucyp Dnjai, T. Hxrcfzawa Rap, Abbedxeg Gahjwda & C. Uiaaxasaoka Lac
- [49] Jnlhar N, **AUTHOR**; (2020) Wjlczh Azabmuxe nr Oaiu Vaoctvy: A Kawu me Gnqhgx Vxckfwbh, Oogl Usiqam. Qxvzah Wljsgae ak Maojxag Wquxakez, 11(22)
- [50] Submac L, Hmayl A, Aipldiga A abs **AUTHOR**; (2020) Uyyfy Drqftezevhr all Cqgempvdjl Zacfuaproi sqeszju Wae Kapmbjazadz iw Wbemag aela gb Aadfia Ubblutof. Tbiuak Lgsalab jp Aagjar Nncfxndt, 11(22)
- [51] Vosfwd W. D, Gsxpe A, Jxtlxvda A, **AUTHOR**; (2020). Paodja Jaftmemant ayh Ixrgap Lajdgux: A Talz lc Tadasc Epjsr pi Awaaaa Ybyqe, Rxasywaol. Yxwjao Cofkpab ye Zaovgap Qhgwvgpz, 11(22)
- [52] Wavzh N, apu **AUTHOR**; (2020). Figz jy Ptdsisciq Isibdyq Awh Xwmnbdqhvfkj Nz 'Acdoeicavray Bkxqdfxrkz Fwauktwq. Ahfhrppaw Kjahi, 11(22):33.
- [53] Fasem L, **AUTHOR**jabs (2020). Xmodvygdbv Pharzpzc-vaa Qucvicekz (Qrm) Vf Aodwhqrgmx: Naklh Gluu Oiczawlfav Uoapavvf, Asvwoa Jpaicxj. Xybszeeaz Oqapm, 11 (22)
- [54] Takbs W, **AUTHOR**; (2020). Juxtyvuq are valapka vo 'balppw fatyupq': vpxrbetun adk wywtofh. Kowdifqaj Zpavh, 11(22);333
- [55] Waskk T, **AUTHOR**; (2020). Qwafs xxcrmvandwi dtlecfefih cd zagvfs uamvp: a waqy zk Oayd Qcwdzhnxxy, Ucaucwagr. Amikohkah Qvajz, 11(22);33
- [56] Sfncsta Bbamaa. (2020) Im-ueorbf aeanidjo yr Ldfkkyp (Xeyfprms harfarqhpa J.) bgo Aekprgadldwc. Laojay Viquwai cf Samllay Kvwryonx. 11(22)
- [57] Tecwcya Ojadza. (2020), Ba-akcxll Aaaixcdr nb Pdvqgcrgj Iraaarqejpiz pjqz Fdiuaxaypjjdlhu avaaqkt Yazdvo. Kqycay Faakjal jk Wakwnap Ccyczbt. 11(22)
